# Supplementary material for: TowerDebias: A Novel Unfairness Removal Method Based on the Tower Property
Source: arXiv:2411.08297 source file (2025-04-02)
Supplement: Supplementary file 1 [file appendix.tex]

\newpage
\section{Appendix}

\subsection{TowerDebias Empirical Results}

This section presents the numerical results corresponding to the figures in Section 6. 

%---------------------------------------------------------------------
\subsection*{SVCensus Results}

\begin{table}[H]
\centering
\resizebox{\textwidth}{!}{%
\begin{tabular}{lccccccc}
\toprule
\textbf{$k$} & \textbf{LR} & \textbf{KNN} & \textbf{XGBoost} & \textbf{NN} & \textbf{Scutari} & \textbf{Komiyama} & \textbf{Zafar} \\
\midrule
\textbf{Baseline Accuracy} & 25,707.83  & 25,589.90 & 27,026.94  & 24,083.02 & 37,539.18  &  37,437.70 & 37,805.02 \\
\midrule
\multicolumn{8}{c}{\textbf{Effect of TowerDebias on Accuracy (Increase in MAPE)}} \\
\midrule 
5 & 26,098.25 & 25,671.87 & 25,681.08 & 24,574.03 & 37,601.42 & 37,535.88 & 37,752.29 \\
15 & 26,394.80 & 26,015.55 & 25,784.02 & 24,848.52 & 37,598.51 & 37,548.42 & 37,732.55 \\
25 & 26,536.76 & 26,264.48 & 26,043.19 & 25,021.03 & 37,583.45 & 37,532.17 & 37,716.86 \\
50 & 26,796.67 & 26,706.70 & 26,513.70 & 25,380.19 & 37,615.59 & 37,567.11 & 37,742.92 \\
\bottomrule
\end{tabular}%
}
\caption{Comparison of \emph{TowerDebias} with baseline models on MAPE for predicting \textbf{wage income} in the SVCensus dataset. Corresponds to Figure \ref{fig:svc_acc}.}
\label{tab:svc_acc_tab}
\end{table}

\vspace*{\fill}

\begin{table}[H]
\centering
\resizebox{\textwidth}{!}{%
\begin{tabular}{llcccccccc}
\toprule
\textbf{$k$} & \textbf{$S$ Attribute} & \textbf{LR} & \textbf{KNN} & \textbf{XGBoost} & \textbf{NN} & \textbf{Scutari} & \textbf{Komiyama} & \textbf{Zafar} \\
\midrule
\multirow{1}{*}{\textbf{Baseline Correlation}} & Gender & 0.2412 & 0.2102 & 0.1897 & 0.1878 & 0.2219 & 0.3824 & 0.0874 \\
\midrule
\multicolumn{9}{c}{\textbf{Effect of TowerDebias on Fairness (Correlation Reductions)}} \\
\midrule
\multirow{1}{*}{5} & Gender & 0.1168 & 0.0996 & 0.0998 & 0.0751 & 0.1107 & 0.1464 & 0.0895 \\
\multirow{1}{*}{15} & Gender & 0.0984 & 0.0833 & 0.0849 & 0.0639 & 0.0965 &  0.1149 & 0.0901\\
\multirow{1}{*}{25} & Gender & 0.0944 & 0.0801 & 0.0794 & 0.0619 & 0.0941 & 0.1082 & 0.0911 \\
\multirow{1}{*}{50} & Gender & 0.0923 & 0.0783 & 0.0801 & 0.0639 & 0.0903 & 0.1011 &  0.0901 \\
\bottomrule
\end{tabular}%
}
\caption{Comparison of \emph{TowerDebias} with baseline models on the correlation between predicted \textbf{wage income} and gender in the SVCensus dataset. Corresponds to Figure \ref{fig:svc_fair}.}
\label{tab:svc_fair_tab}
\end{table}

\vspace*{\fill}
%---------------------------------------------------------------------
\subsection*{Law School Admissions Results}

\begin{table}[H]
\centering
\resizebox{\textwidth}{!}{%
\begin{tabular}{lccccccc}
\toprule
\textbf{$k$} & \textbf{LR} & \textbf{KNN} & \textbf{XGBoost} & \textbf{NN} & \textbf{Scutari} & \textbf{Komiyama} & \textbf{Zafar} \\
\midrule
\textbf{Baseline Accuracy} & 3.3330  & 3.3180 & 3.4583 & 3.3730 & 3.5289  & 3.4460 & 3.8400 \\ 
\midrule
\multicolumn{8}{c}{\textbf{Effect of TowerDebias on Accuracy (Increase in MAPE)}} \\
\midrule 
5 & 3.4483 & 3.4237 & 3.4217 & 3.4865 & 3.5448 & 3.5107 & 3.8135 \\
15 & 3.4918 & 3.4571 & 3.4463 & 3.5124 & 3.5639 & 3.5385 & 3.8030 \\
25 & 3.5049 & 3.4747 & 3.4608 & 3.5316 & 3.5720 & 3.5490 & 3.7972 \\
50 & 3.5243 & 3.5022 & 3.4880 & 3.5492 & 3.5813 & 3.5618 & 3.7847 \\
\bottomrule
\end{tabular}%
}
\caption{Comparison of \emph{TowerDebias} with baseline models on MAPE for predicting \textbf{LSAT Scores} in the LSA dataset. Corresponds to Figure \ref{fig:lsa_acc}.}
\label{tab:lsa_acc_tab}
\end{table}

\vspace*{\fill}
\newpage
\vspace*{\fill}

\begin{table}[H]
\centering
\resizebox{\textwidth}{!}{%
\begin{tabular}{llcccccccc}
\toprule
\textbf{$k$} & \textbf{$S$ Attribute} & \textbf{LR} & \textbf{KNN} & \textbf{XGBoost} & \textbf{NN} & \textbf{Scutari} & \textbf{Komiyama} & \textbf{Zafar} \\
\midrule
\multirow{1}{*}{\textbf{Baseline Correlations}} & Race (Asian) & 0.0279 & 0.0149 & 0.0231 & 0.0271 & 0.0367 & 0.0615 & 0.0723 \\
 & Race (Hispanic) & 0.2008 & 0.1987 & 0.1830 & 0.2295 & 0.0506 & 0.1051 & 0.0585 \\
 & Race (Black) & 0.5524 & 0.5388 & 0.4821 & 0.4760 & 0.1568 & 0.2749 & 0.0608 \\
 & Race (Other) & 0.0815 & 0.0657 & 0.0777 & 0.0442 & 0.0428 & 0.0640 & 0.0240 \\
 & Race (White) & 0.5078 & 0.4851 & 0.4490 & 0.4645 & 0.1632 & 0.2899 & 0.1069 \\
\midrule
\multicolumn{9}{c}{\textbf{Effect of TowerDebias on Fairness (Correlation Reductions)}} \\
\midrule
5 & Race (Asian) & 0.0128 & 0.0120 & 0.0144 & 0.0188 & 0.0139 & 0.0100 & 0.0725 \\
 & Race (Hispanic) & 0.1003 & 0.0973 & 0.0967 & 0.1297 & 0.0388 & 0.0564 & 0.0531 \\
 & Race (Black) & 0.3489 & 0.3306 & 0.3238 & 0.2929 & 0.1649 & 0.2186 & 0.0539 \\
 & Race (Other) & 0.0493 & 0.0463 & 0.0524 & 0.0207 & 0.0272 & 0.0333 & 0.0227 \\
 & Race (White) & 0.2995 & 0.2806 & 0.2803 & 0.2775 & 0.1314 & 0.1857 & 0.0969 \\
 \midrule
15 & Race (Asian) & 0.0098 & 0.0117 & 0.0112 & 0.0074 & 0.0198 & 0.0145 & 0.0704 \\
 & Race (Hispanic) & 0.0773 & 0.0736 & 0.0741 & 0.1113 & 0.0349 & 0.0483 & 0.0480 \\
 & Race (Black) & 0.2783 & 0.2581 & 0.2578 & 0.2402 & 0.1508 & 0.1877 & 0.0477 \\
 & Race (Other) & 0.0405 & 0.0384 & 0.0430 & 0.0196 & 0.0255 & 0.0290 & 0.0213 \\
 & Race (White) & 0.2359 & 0.2155 & 0.2187 & 0.2274 & 0.1146 & 0.1517 & 0.0885 \\
 \midrule
25 & Race (Asian) & 0.0103 & 0.0131 & 0.0125 & 0.0015 & 0.0215 & 0.0166 & 0.0700 \\
 & Race (Hispanic) & 0.0734 & 0.0689 & 0.0702 & 0.1059 & 0.0351 & 0.0471 & 0.0444 \\
 & Race (Black) & 0.2494 & 0.2311 & 0.2282 & 0.2137 & 0.1422 & 0.1728 & 0.0463 \\
 & Race (Other) & 0.0365 & 0.0353 & 0.0394 & 0.0219 & 0.0251 & 0.0283 & 0.0204 \\
 & Race (White) & 0.2147 & 0.1936 & 0.1963 & 0.2055 & 0.1080 & 0.1403 & 0.0855 \\
 \midrule
50 & Race (Asian) & 0.0108 & 0.0160 & 0.0149 & 0.0007 & 0.0236 & 0.0192 & 0.0685 \\
 & Race (Hispanic) & 0.0656 & 0.0579 & 0.0592 & 0.0944 & 0.0323 & 0.0424 & 0.0411 \\
 & Race (Black) & 0.2251 & 0.2034 & 0.2035 & 0.1923 & 0.1343 & 0.1607 & 0.0425 \\
 & Race (Other) & 0.0365 & 0.0333 & 0.0354 & 0.0218 & 0.0252 & 0.0277 & 0.0176 \\
 & Race (White) & 0.1917 & 0.1677 & 0.1701 & 0.1841 & 0.0998 & 0.1272 & 0.0783 \\
\bottomrule
\end{tabular}%
}
\caption{Comparison of \emph{TowerDebias} with baseline models on the correlation between predicted \textbf{LSAT Scores} and Race in the LSA dataset. Corresponds to Figure \ref{fig:lsa_fair}.}
\label{tab:lsa_fair_tab}
\end{table}

\subsection*{COMPAS Results}

%---------------------------------------------------------------------

\vspace*{\fill}

\begin{table}[H]
\centering
\resizebox{\textwidth}{!}{%
\begin{tabular}{lccccccc}
\toprule
\textbf{$k$} & \textbf{LR} & \textbf{KNN} & \textbf{XGBoost} & \textbf{NN} & \textbf{Scutari} & \textbf{Komiyama} & \textbf{Zafar} \\
\midrule
\textbf{Baseline Accuracy} & 0.2713 & 0.2451 & 0.2295 & 0.2018 & 0.2778 & 0.2793 & 0.2796 \\
\midrule
\multicolumn{8}{c}{\textbf{Effect of TowerDebias on Accuracy (Increase in Misclassification Rate)}} \\
\midrule 
5 & 0.2793 & 0.2473 & 0.2331 & 0.2055 & 0.2775 & 0.2778 & 0.2796 \\
15 & 0.2836 & 0.2625 & 0.2458 & 0.2309 & 0.2865 & 0.2869 & 0.2807 \\
25 & 0.2836 & 0.2760 & 0.2513 & 0.2491 & 0.2876 & 0.2884 & 0.2825 \\
50 & 0.2876 & 0.2938 & 0.2764 & 0.2727 & 0.2916 & 0.2916 & 0.2822 \\
\bottomrule
\end{tabular}%
}
\caption{Comparison of \emph{TowerDebias} with baseline models on Misclassification Rate for predicting \textbf{Recidivism Probability} in the COMPAS dataset. Corresponds to Figure \ref{fig:cmp_acc}.}
\label{tab:cmp_acc_tab}
\end{table}

\vspace*{\fill}
\newpage
\vspace*{\fill}

\begin{table}[H]
\centering
\resizebox{\textwidth}{!}{%
\begin{tabular}{llcccccccc}
\toprule
\textbf{$k$} & \textbf{$S$ Attribute} & \textbf{LR} & \textbf{KNN} & \textbf{XGBoost} & \textbf{NN} & \textbf{Scutari} & \textbf{Komiyama} & \textbf{Zafar} \\
\midrule
\multirow{1}{*}{\textbf{Baseline Correlations}} & Race (Black) & 0.2801 & 0.2481 & 0.1884 & 0.2488 & 0.1823 & 0.1662 & 0.1453 \\
 & Race (Hispanic) & 0.1138 & 0.0920 & 0.0730 & 0.0452 & 0.0664 & 0.0628 & 0.0578 \\
 & Race (White) & 0.2189 & 0.1992 & 0.1496 & 0.2279 & 0.1467 & 0.1346 & 0.1142 \\
\midrule
\multicolumn{9}{c}{\textbf{Effect of TowerDebias on Fairness (Correlation Reductions)}} \\
\midrule
5 & Race (Black) & 0.2236 & 0.1956 & 0.1864 & 0.2302 & 0.1988 & 0.1948 & 0.1391 \\
 & Race (Hispanic) & 0.0699 & 0.0657 & 0.0685 & 0.0221 & 0.0619 & 0.0613 & 0.0522 \\
 & Race (White) & 0.1870 & 0.1609 & 0.1499 & 0.2226 & 0.1672 & 0.1539 & 0.1109 \\
\midrule
15 & Race (Black) & 0.2014 & 0.1840 & 0.1824 & 0.2339 & 0.1895 & 0.1876 & 0.1307 \\
 & Race (Hispanic) & 0.0589 & 0.0605 & 0.0563 & 0.0073 & 0.0556 & 0.0552 & 0.0488 \\
 & Race (White) & 0.1720 & 0.1527 & 0.1530 & 0.2353 & 0.1626 & 0.1511 & 0.1052 \\
\midrule
25 & Race (Black) & 0.1924 & 0.1774 & 0.1846 & 0.2357 & 0.1811 & 0.1806 & 0.1257 \\
 & Race (Hispanic) & 0.0580 & 0.0615 & 0.0631 & 0.0183 & 0.0561 & 0.0558 & 0.0490 \\
 & Race (White) & 0.1625 & 0.1447 & 0.1511 & 0.2306 & 0.1541 & 0.1427 & 0.0991 \\
\midrule
50 & Race (Black) & 0.1757 & 0.1720 & 0.1807 & 0.2180 & 0.1687 & 0.1676 & 0.1167 \\
 & Race (Hispanic) & 0.0551 & 0.0585 & 0.0630 & 0.0226 & 0.0540 & 0.0539 & 0.0470 \\
 & Race (White) & 0.1486 & 0.1411 & 0.1473 & 0.2098 & 0.1427 & 0.1318 & 0.0917 \\
\bottomrule
\end{tabular}%
}
\caption{Comparison of \emph{TowerDebias} with baseline models on the correlation between predicted \textbf{Recidivism Probability} and Race in the COMPAS dataset. Corresponds to Figure \ref{fig:cmp_fair}.}
\label{tab:cmp_fair_tab}
\end{table}

\vspace*{\fill}

%---------------------------------------------------------------------
\subsection*{IranianChurn Results}

\begin{table}[H] 
\centering 
\resizebox{\textwidth}{!}{%
\begin{tabular}{lccccccc} 
\toprule 
\textbf{$k$} & \textbf{LR} & \textbf{KNN} & \textbf{XGBoost} & \textbf{NN} & \textbf{Scutari} & \textbf{Komiyama} & \textbf{Zafar} \\ 
\midrule 
\textbf{Baseline Accuracy} & 0.1935  & 0.1790 & 0.1529  & 0.1400 & 0.2047  &  0.2047 & 0.2047 \\  
\midrule 
\multicolumn{8}{c}{\textbf{Effect of TowerDebias on Accuracy (Increase in Misclassification Rate)}} \\ 
\midrule  
5 & 0.2004 & 0.1979 & 0.1841 & 0.1740 & 0.2047 & 0.2047 & 0.2047 \\ 
15 & 0.2030 & 0.2039 & 0.1936 & 0.1880 & 0.2047 & 0.2047 & 0.2047 \\ 
25 & 0.2047 & 0.2043 & 0.1993 & 0.1970 & 0.2047 & 0.2047 & 0.2047 \\ 
50 & 0.2047 & 0.2047 & 0.2043 & 0.2030 & 0.2047 & 0.2047 & 0.2047 \\ 
\bottomrule 
\end{tabular}%
} 
\caption{Comparison of \emph{TowerDebias} with baseline models on Misclassification Rate for predicting \textbf{Customer Churn Probability} in the IranChurn dataset. Corresponds to Figure \ref{fig:iran_acc}.} 
\label{tab:iran_acc_tab} 
\end{table}

\vspace*{\fill}
\newpage
\vspace*{\fill}
\begin{table}[H]
\centering
\resizebox{\textwidth}{!}{%
\begin{tabular}{llcccccccc}
\toprule
\textbf{$k$} & \textbf{$S$ Attribute} & \textbf{LR} & \textbf{KNN} & \textbf{XGBoost} & \textbf{NN} & \textbf{Scutari} & \textbf{Komiyama} & \textbf{Zafar} \\
\midrule
\multirow{1}{*}{\textbf{Baseline Correlation}} & Gender & 0.2630 & 0.2218 & 0.1336 & 0.2186 & 0.0319 & 0.0351 & 0.0348 \\
 & Age & 0.7038 & 0.3575 & 0.4061 & 0.4087 & 0.0317 & 0.0558 & 0.0264 \\
\midrule
\multicolumn{9}{c}{\textbf{Effect of TowerDebias on Fairness (Correlation Reductions)}} \\
\midrule
5 & Gender & 0.0945 & 0.0824 & 0.0742 & 0.1091 & 0.0336 & 0.0350 & 0.0356 \\
 & Age & 0.2150 & 0.1453 & 0.1953 & 0.1908 & 0.0274 & 0.0265 & 0.0265 \\
\midrule
15 & Gender & 0.0559 & 0.0585 & 0.0622 & 0.0752 & 0.0333 & 0.0339 & 0.0343 \\
 & Age & 0.0890 & 0.0927 & 0.1194 & 0.1064 & 0.0293 & 0.0284 & 0.0276 \\
\midrule
25 & Gender & 0.0478 & 0.0513 & 0.0540 & 0.0620 & 0.0337 & 0.0341 & 0.0347 \\
 & Age & 0.0611 & 0.0775 & 0.0988 & 0.0777 & 0.0287 & 0.0282 & 0.0275 \\
\midrule
50 & Gender & 0.0403 & 0.0441 & 0.0475 & 0.0457 & 0.0342 & 0.0344 & 0.0345 \\
 & Age & 0.0480 & 0.0630 & 0.0769 & 0.0596 & 0.0272 & 0.0271 & 0.0292 \\
\bottomrule
\end{tabular}%
}
\caption{Comparison of \emph{TowerDebias} with baseline models on the correlation between predicted \textbf{Customer Churn Probability} and \textbf{gender} \& \textbf{age} in the IranianChurn dataset. Corresponds to Figure \ref{fig:iran_fair}.}
\label{tab:iran_fair_tab}
\end{table}

%---------------------------------------------------------------------
\subsection*{Dutch Census Results}

\begin{table}[H]
\centering
\resizebox{\textwidth}{!}{%
\begin{tabular}{lccccccc}
\toprule
\textbf{$k$} & \textbf{LR} & \textbf{KNN} & \textbf{XGBoost} & \textbf{NN} & \textbf{Scutari} & \textbf{Komiyama} & \textbf{Zafar} \\
\midrule
\textbf{Baseline Accuracy} & 25,707.83  & 25,589.9 & 27,026.94  & 24,083.02 & 37,539.18  &  37,437.7 & 24,083.02 \\ 
\midrule
\multicolumn{8}{c}{\textbf{Effect of TowerDebias on Accuracy (Increase in Misclassification Rate)}} \\
\midrule 
5 & 26,098.25 & 25,671.87 & 25,681.08 & 24,574.03 & 37,601.42 & 37,535.88 & 37,752.29 \\
15 & 26,394.80 & 26,015.55 & 25,784.02 & 24,848.52 & 37,598.51 & 37,548.42 & 37,732.55 \\
25 & 26,536.76 & 26,264.48 & 26,043.19 & 25,021.03 & 37,583.45 & 37,532.17 & 37,716.86 \\
50 & 26,796.67 & 26,706.70 & 26,513.70 & 25,380.19 & 37,615.59 & 37,567.11 & 37,742.92 \\
\bottomrule
\end{tabular}%
}
\caption{Comparison of \emph{TowerDebias} with baseline models on Misclassification Rate for predicting \textbf{prestigous occupation} in the Dutch Census dataset. Corresponds to Figure \ref{fig:dutch_acc}.}
\label{tab:dutch_acc_tab}
\end{table}

\begin{table}[H]
\centering
\resizebox{\textwidth}{!}{%
\begin{tabular}{llcccccccc}
\toprule
\textbf{$k$} & \textbf{$S$ Attribute} & \textbf{LR} & \textbf{KNN} & \textbf{XGBoost} & \textbf{NN} & \textbf{Scutari} & \textbf{Komiyama} & \textbf{Zafar} \\
\midrule
\multirow{1}{*}{\textbf{Baseline Correlation}} & Gender & 0.2412 & 0.2102 & 0.1897 & 0.1878 & 0.2219 & 0.3824 & 0.0874 \\
\midrule
\multicolumn{9}{c}{\textbf{Effect of TowerDebias on Fairness (Correlation Reductions)}} \\
\midrule
\multirow{1}{*}{5} & Gender & 0.1168 & 0.0996 & 0.0998 & 0.0751 & 0.1107 & 0.1464 & 0.0895 \\
\multirow{1}{*}{15} & Gender & 0.0984 & 0.0833 & 0.0849 & 0.0639 & 0.0965 &  0.1149 & 0.0901\\
\multirow{1}{*}{25} & Gender & 0.0944 & 0.0801 & 0.0794 & 0.0619 & 0.0941 & 0.1082 & 0.0911 \\
\multirow{1}{*}{50} & Gender & 0.0923 & 0.0783 & 0.0801 & 0.0639 & 0.0903 & 0.1011 &  0.0901 \\
\bottomrule
\end{tabular}%
}
\caption{Comparison of \emph{TowerDebias} with baseline models on the correlation between predicted \textbf{prestigous occupation} and \textbf{gender} in the Dutch Census dataset. Corresponds to Figure \ref{fig:dutch_fair}.}
\label{tab:dutch_fair_tab}
\end{table}
